# Supplementary material for: Thermodynamic speed limits for co-evolving systems
Source: arXiv:2107.12471 ancillary file (2021-12-04)
Supplement: Supplementary file 1 [file speed_limits_for_mpps_supp.pdf]

# Supplemental Material for
# "Thermodynamic speed limits for multiple, co-evolving systems"

Farita Tasnim and David Wolpert

We derive our new SLTs in full detail in Sections S1 and S2. We prove that a subsystem's contribution to the global dynamical activity equals its contribution to the local dynamical activity of any unit of which it is a part in Section S3. In Section S4, we discuss how our results extend the applicability of thermodynamic speed limits to systems characterized by local, rather than global, interactions. In doing so, we establish thermodynamic consistency of our results for systems whose dynamics are defined by local, rather than global, Hamiltonians. In Section S5, we show that each of the subsystem-indexed contributions to the global EP follows an integral fluctuation theorem. In Section S6, we note that the global SLT also applies to subsets of subsystems, or units, that evolve according to their own CTMC; this leads to what we call "unit-local SLTs". In Section S7, we prove that the strongest of a generalized form of the SLT that involves a linear combination of unit-local thermodynamic properties is given by the unit-local SLT for the system's slowest-evolving unit. In Section S8, we consider the SLTs as bounds on the space of distributions that a system can access within a given time. In particular, we show that the unit-local SLTs together more tightly restrict (than the global SLT) this space of final joint distributions for a pair of independently evolving spins. In Section S9, we derive maximum and minimum speeds of evolution for Bayes' Nets, which are a type of MPP for which the state transitions occur according to a global clock. Finally, in Section S10, we derive lower bounds on the difference between the EP rate and the rate at which one unit "learns" about another using counterfactual thermodynamic quantities.

## S1 Derivation of Eqs. (18) and (19)

To begin, we note that subsystem $i$'s contribution to the EP rate obeys the following inequality:

$$\langle \dot{\zeta}^i_{\mathcal{N}}(t)\rangle = \sum_{x',x} K_x^{x'}(i;t)p_{x'}(t)\ln\left[\frac{K_x^{x'}(i;t)p_{x'}(t)}{K_{x'}^{x}(i;t)p_x(t)}\right] \tag{S1}$$

$$= \frac{1}{2}\sum_{x}\sum_{x'\neq x}\Big(K_x^{x'}(i;t)p_{x'}(t) - K_{x'}^{x}(i;t)p_x(t)\Big)\ln\left[\frac{K_x^{x'}(i;t)p_{x'}(t)}{K_{x'}^{x}(i;t)p_x(t)}\right] \tag{S2}$$

$$= \frac{1}{2}\sum_{x'_{-i}}\sum_{x_i}\sum_{x'_i\neq x_i}\left(K_{x_i,x'_{-i}}^{x'_i,x'_{-i}}(i;t)p_{x'_i,x'_{-i}}(t) - K_{x'_i,x'_{-i}}^{x_i,x'_{-i}}(i;t)p_{x_i,x'_{-i}}(t)\right)\ln\left[\frac{K_{x_i,x'_{-i}}^{x'_i,x'_{-i}}(i;t)p_{x'_i,x'_{-i}}(t)}{K_{x'_i,x'_{-i}}^{x_i,x'_{-i}}(i;t)p_{x_i,x'_{-i}}(t)}\right] \tag{S3}$$

$$\geq \sum_{x'_{-i}}\sum_{x_i}\sum_{x'_i\neq x_i}\frac{\left(K_{x_i,x'_{-i}}^{x'_i,x'_{-i}}(i;t)p_{x'_i,x'_{-i}}(t) - K_{x'_i,x'_{-i}}^{x_i,x'_{-i}}(i;t)p_{x_i,x'_{-i}}(t)\right)^2}{K_{x_i,x'_{-i}}^{x'_i,x'_{-i}}(i;t)p_{x'_i,x'_{-i}}(t) + K_{x'_i,x'_{-i}}^{x_i,x'_{-i}}(i;t)p_{x_i,x'_{-i}}(t)} \tag{S4}$$

Similarly,

$$\langle \dot{\zeta}^i_{\omega}(t)\rangle \geq \sum_{x'_{\omega\setminus i}}\sum_{x_i}\sum_{x'_i\neq x_i}\frac{\left(K_{x_i,x'_{\omega\setminus i}}^{x'_i,x'_{\omega\setminus i}}(i;t)p_{x'_i,x'_{\omega\setminus i}}(t) - K_{x'_i,x'_{\omega\setminus i}}^{x_i,x'_{\omega\setminus i}}(i;t)p_{x_i,x'_{\omega\setminus i}}(t)\right)^2}{K_{x_i,x'_{\omega\setminus i}}^{x'_i,x'_{\omega\setminus i}}(i;t)p_{x'_i,x'_{\omega\setminus i}}(t) + K_{x'_i,x'_{\omega\setminus i}}^{x_i,x'_{\omega\setminus i}}(i;t)p_{x_i,x'_{\omega\setminus i}}(t)} \tag{S5}$$

These inequalities hold because $(a-b)\ln\frac{a}{b} \geq \frac{(a-b)^2}{(a+b)}$ for all positive $a$ and $b$, as pointed out in [9]. We can then use the fact that $\frac{d}{dt}p_x(t) = \sum_{i\in\mathcal{N}} \frac{d}{dt}p_{x_i}(t)$ (which follows from Eqs. (2), (3), and (7)) to bound the global total variation distance as follows:

$$\sum_x \left|\frac{d}{dt}p_x(t)\right| = \sum_x \left|\sum_{x'\neq x}\sum_{i\in\mathcal{N}}\left(K_x^{x'}(i;t)p_{x'}(t) - K_{x'}^{x}(i;t)p_x(t)\right)\right| \tag{S6}$$

$$\leq \sum_{i\in\mathcal{N}}\sum_{x_i,x_{-i}}\left|\sum_{x'_{-i}}\sum_{x'_i\neq x_i}\left(K_{x_i,x'_{-i}}^{x'_i,x'_{-i}}(i;t)p_{x'_i,x'_{-i}}(t) - K_{x'_i,x'_{-i}}^{x_i,x'_{-i}}(i;t)p_{x_i,x'_{-i}}(t)\right)\right|$$

$$= \sum_{i\in\mathcal{N}}\sum_{x_i}\left|\sum_{x'_{-i}}\sum_{x'_i\neq x_i}\left(K_{x_i,x'_{-i}}^{x'_i,x'_{-i}}(i;t)p_{x'_i,x'_{-i}}(t) - K_{x'_i,x'_{-i}}^{x_i,x'_{-i}}(i;t)p_{x_i,x'_{-i}}(t)\right)\right| \tag{S7}$$

$$\leq \sum_{i\in\mathcal{N}}\sum_{x_i}\sqrt{\left(\sum_{x'_{-i}}\sum_{x'_i\neq x_i}\frac{\left(K_{x_i,x'_{-i}}^{x'_i,x'_{-i}}(i;t)p_{x'_i,x'_{-i}}(t) - K_{x'_i,x'_{-i}}^{x_i,x'_{-i}}(i;t)p_{x_i,x'_{-i}}(t)\right)^2}{K_{x_i,x'_{-i}}^{x'_i,x'_{-i}}(i;t)p_{x'_i,x'_{-i}}(t) + K_{x'_i,x'_{-i}}^{x_i,x'_{-i}}(i;t)p_{x_i,x'_{-i}}(t)}\right)\left(\sum_{x'_{-i}}\sum_{x'_i\neq x_i}K_{x_i,x'_{-i}}^{x'_i,x'_{-i}}(i;t)p_{x'_i,x'_{-i}}(t) + K_{x'_i,x'_{-i}}^{x_i,x'_{-i}}(i;t)p_{x_i,x'_{-i}}(t)\right)} \tag{S8}$$

$$\leq \sum_{i\in\mathcal{N}}\sqrt{\left(\sum_{x'_{-i}}\sum_{x_i}\sum_{x'_i\neq x_i}\frac{\left(K_{x_i,x'_{-i}}^{x'_i,x'_{-i}}(i;t)p_{x'_i,x'_{-i}}(t) - K_{x'_i,x'_{-i}}^{x_i,x'_{-i}}(i;t)p_{x_i,x'_{-i}}(t)\right)^2}{K_{x_i,x'_{-i}}^{x'_i,x'_{-i}}(i;t)p_{x'_i,x'_{-i}}(t) + K_{x'_i,x'_{-i}}^{x_i,x'_{-i}}(i;t)p_{x_i,x'_{-i}}(t)}\right)\left(\sum_{x'_{-i}}\sum_{x_i}\sum_{x'_i\neq x_i}K_{x_i,x'_{-i}}^{x'_i,x'_{-i}}(i;t)p_{x'_i,x'_{-i}}(t) + K_{x'_i,x'_{-i}}^{x_i,x'_{-i}}(i;t)p_{x_i,x'_{-i}}(t)\right)} \tag{S9}$$

$$\leq \sum_{i\in\mathcal{N}}\sqrt{2\langle\dot{\zeta}^i_{\mathcal{N}}(t)\rangle\mathcal{A}^i(t)} \tag{S10}$$

Then, integrating over time,

$$\mathcal{L}(p_x(0),p_x(\tau)) \leq \sum_x\int_0^\tau dt\left|\frac{d}{dt}p_x(t)\right| \tag{S11}$$

$$\leq \sum_{i\in\mathcal{N}}\int_0^\tau dt\sqrt{2\langle\dot{\zeta}^i_{\mathcal{N}}(t)\rangle\mathcal{A}^i(t)} \tag{S12}$$

$$\leq \sum_{i\in\mathcal{N}}\sqrt{2\tau\langle\zeta^i_{\mathcal{N}}(\tau)\rangle\langle\mathcal{A}^i\rangle_\tau} \tag{S13}$$

where we have used the Cauchy-Schwartz inequality in the step from Eq. (S8) to Eq. (S9) and in the step from Eq. (S12) to Eq. (S13). This leads to the speed limit in Eq. (18).

*Mutatis mutandis*, we can follow a similar exercise for the subsystems in a unit (same steps as above derivation but with all $\mathcal{N}$ replaced with $\omega$, with the state space limited to $x_\omega$ instead of $x$, and with using Eq. (S5) instead of Eq. (S4)) to obtain the speed limit in Eq. (19). One such speed limit holds for each unit $\omega \in \mathcal{N}^{**}$.

## S2 Derivation of Eq. (20)

We can bound the marginal total variation distance of subsystem $i$ as follows:

$$\sum_{x_i}\left|\frac{d}{dt}p_{x_i}(t)\right| \leq \sum_{x_i}\left|\sum_{x'_{-i}}\sum_{x'_i\neq x_i}\left(K_{x_i,x'_{-i}}^{x'_i,x'_{-i}}(i;t)p_{x'_i,x'_{-i}}(t) - K_{x'_i,x'_{-i}}^{x_i,x'_{-i}}(i;t)p_{x_i,x'_{-i}}(t)\right)\right| \tag{S14}$$

$$\leq \sum_{x_i} \sqrt{\left( \sum_{x'_{-i}} \sum_{x'_i \neq x_i} \frac{\left( K^{x'_i, x'_{-i}}_{x_i, x'_{-i}}(i;t) p_{x'_i, x'_{-i}}(t) - K^{x_i, x'_{-i}}_{x'_i, x'_{-i}}(i;t) p_{x_i, x'_{-i}}(t) \right)^2}{K^{x'_i, x'_{-i}}_{x_i, x'_{-i}}(i;t) p_{x'_i, x'_{-i}}(t) + K^{x_i, x'_{-i}}_{x'_i, x'_{-i}}(i;t) p_{x_i, x'_{-i}}(t)} \right) \left( \sum_{x'_{-i}} \sum_{x'_i \neq x_i} K^{x'_i, x'_{-i}}_{x_i, x'_{-i}}(i;t) p_{x'_i, x'_{-i}}(t) + K^{x_i, x'_{-i}}_{x'_i, x'_{-i}}(i;t) p_{x_i, x'_{-i}}(t) \right)} \tag{S15}$$

$$\leq \sqrt{\left( \sum_{x'_{-i}} \sum_{x_i} \sum_{x'_i \neq x_i} \frac{\left( K^{x'_i, x'_{-i}}_{x_i, x'_{-i}}(i;t) p_{x'_i, x'_{-i}}(t) - K^{x_i, x'_{-i}}_{x'_i, x'_{-i}}(i;t) p_{x_i, x'_{-i}}(t) \right)^2}{K^{x'_i, x'_{-i}}_{x_i, x'_{-i}}(i;t) p_{x'_i, x'_{-i}}(t) + K^{x_i, x'_{-i}}_{x'_i, x'_{-i}}(i;t) p_{x_i, x'_{-i}}(t)} \right) \left( \sum_{x'_{-i}} \sum_{x_i} \sum_{x'_i \neq x_i} K^{x'_i, x'_{-i}}_{x_i, x'_{-i}}(i;t) p_{x'_i, x'_{-i}}(t) + K^{x_i, x'_{-i}}_{x'_i, x'_{-i}}(i;t) p_{x_i, x'_{-i}}(t) \right)} \tag{S16}$$

$$\leq \sqrt{2 \langle \dot{\zeta}^i_{\mathcal{N}}(t) \rangle \mathcal{A}^i(t)} \tag{S17}$$

Then, integrating over time,

$$\mathcal{L}(p_{x_i}(0), p_{x_i}(\tau)) \leq \sum_{x_i} \int_0^\tau dt \left| \frac{d}{dt} p_{x_i}(t) \right| \tag{S18}$$

$$\leq \int_0^\tau dt \sqrt{2 \langle \dot{\zeta}^i_{\mathcal{N}}(t) \rangle \mathcal{A}^i(t)} \tag{S19}$$

$$\leq \sqrt{2 \tau \langle \zeta^i_{\mathcal{N}}(\tau) \rangle \langle \mathcal{A}^i \rangle_\tau} \tag{S20}$$

where we have used the Cauchy-Schwartz inequality in the step from Eq. (S15) to Eq. (S16) and in the step from Eq. (S19) to Eq. (S20). One such speed limit like this holds for each subsystem $i \in \mathcal{N}$. Similarly, let's consider any unit $\omega$ such that $i \in \omega$. If we replace all $-i$ with $\omega \backslash i$ in the above derivation, we obtain

$$\forall \omega \in \mathcal{N}^\dagger | i \in \omega : \ \mathcal{L}(p_{x_i}(0), p_{x_i}(\tau)) \leq \sqrt{2 \tau \langle \zeta^i_\omega(\tau) \rangle \langle \mathcal{A}^i \rangle_\tau} \tag{S21}$$

Noting that the minimum of the RHS of Eq. (S21) will provide the tightest bound, we arrive at the speed limit in Eq. (20). Remember that $\mathcal{N}^\dagger = \mathcal{N}^{**} \cup \mathcal{N}$, so that Eq. (S21) subsumes Eq. (S20).

## S3 Proof that a Subsystem's Contribution to the Global Dynamical Activity Equals its Contribution to any Local Dynamical Activity

We show that subsystem $i$'s contribution to the global dynamical activity is equal to its contribution to the local dynamical activity of any

$$\mathcal{A}^i_{\mathcal{N}}(t) = \sum_{x'_{-i}} \sum_{x_i} \sum_{x'_i \neq x_i} K^{x'_i, x'_{-i}}_{x_i, x'_{-i}}(i;t) p_{x'_i, x'_{-i}}(t) \tag{S22}$$

$$= \sum_{x'_{-\omega}} \sum_{x'_{\omega \backslash i}} \sum_{x_i} \sum_{x'_i \neq x_i} K^{x'_i, x'_{\omega \backslash i}, x'_{-\omega}}_{x_i, x'_{\omega \backslash i}, x'_{-\omega}}(i;t) p_{x'_i, x'_{\omega \backslash i}, x'_{-\omega}}(t) \tag{S23}$$

$$= \sum_{x'_{\omega \backslash i}} \sum_{x_i} \sum_{x'_i \neq x_i} K^{x'_i, x'_{\omega \backslash i}}_{x_i, x'_{\omega \backslash i}}(i;t) p_{x'_i, x'_{\omega \backslash i}}(t) \tag{S24}$$

$$= \mathcal{A}^i_\omega(t) \tag{S25}$$

where in the jump from Eq. (S24) to Eq. (S25), we utilized Eq. (6) from the main text, as well as the extension of that equation for a unit $\omega$ and any subsystem $i \in \omega$:

$$K^{x'_\omega}_{x_\omega}(i;t) = K^{x'_{r(i;t)}}_{x_{r(i;t)}}(i;t) \, \delta(x'_{-r(i;t)}, x_{-r(i;t)}) \tag{S26}$$

Hence,

$$\mathcal{A}^i_{\mathcal{N}}(t) = \mathcal{A}^i_{\omega}(t) = \mathcal{A}^i(t) \tag{S27}$$

Intuitively, this makes sense because the dynamical activity is interpreted as the frequency of state transitions. In an MPP, there are no simultaneous state transitions. Accordingly, the contribution to any dynamical activity due a subsystem $i$ will be the frequency of state transitions in the state of subsystem $i$, which only depends on $r(i)$. Since $r(i) \in \omega$ for any unit $\omega \in \mathcal{N}^\dagger \mid i \in \omega$, the probability flows caused by state transitions in $i$ are independent of which unit one uses to contextualize those probability flows.

# S4 Thermodynamic Consistency of the MPP SLTs and Different Types of Local-Detailed Balance

We emphasize that, unlike the global SLT, our MPP SLTs extend in a physically meaningful way to experimental scenarios in which the rate matrices are defined with local rather than global Hamiltonians. To establish this claim, we first outline the different types of local detailed balance possible in an MPP.

Local detailed balance (LDB), as is standard in literature, means that the entire system obeys the following relation for arbitrary state transitions (in any subsystem $i$) using the same global Hamiltonian:

$$\ln\left[\frac{K_x^{x'}(i;t)}{K_{x'}^{x}(i;t)}\right] = \beta_i \left(H_{x'}(t) - H_x(t)\right) \tag{S28}$$

For an MPP, we call this **global LDB (GLDB)**.

In a system consisting of multiple, co-evolving subsystems, however, it is often impossible to write down a global Hamiltonian in a thermodynamically consistent way, e.g., as could be caused by non-reciprocal dependency constraints [7, 8, 2, 12, 14]. Therefore, we also define the following types of LDB that can establish thermodynamic consistency for MPPs whose rate matrices are constrained by non-global Hamiltonians.

**Unit LDB (ULDB)** means that each unit $\omega$ obeys LDB for state transitions (of any subsystem $i$ in that unit) using a unit-specific local Hamiltonian, which can only depend on the states of subsystems within that unit:

$$\ln\left[\frac{K_x^{x'}(i;t)}{K_{x'}^{x}(i;t)}\right] = \beta_i \left(H_{x'_\omega}(\omega;t) - H_{x_\omega}(\omega;t)\right) \tag{S29}$$

ULDB does not follow from GLDB.

**Subsystem LDB (SLDB)** means that each subsystem $i$ obeys LDB for its own state transitions using its own local Hamiltonian, which can only depend on the states of the subsystems ($j \in r(i)$) that affect $i$:

$$\ln\left[\frac{K_x^{x'}(i;t)}{K_{x'}^{x}(i;t)}\right] = \beta_i \left(H_{x'_{r(i)}}(i;t) - H_{x_{r(i)}}(i;t)\right) \tag{S30}$$

for some local Hamiltonians $H_{x_{r(i)}}(i;t)$. SLDB does not follow from ULDB or GLDB.

Mathematically, the global SLT from [9] is valid for all classical stochastic processes. However, when a system obeys only SLDB, e.g., if it is defined using local Hamiltonians, there does not necessarily exist a global Hamiltonian $H_x(t)$ that is consistent with all of the local Hamiltonians. Therefore, the quantity $\langle \sigma^{\mathcal{N}}(t)\rangle$, and thus the global SLT, is not physically meaningful in this context because the function for the global entropy flow (EF) breaks down (Eq. (5) from [9] becomes nonphysical).

Here we show that the thermodynamic consistency of our MPP SLTs does not require GLDB. Instead, SLDB is sufficient. Therefore, our results vastly open up the experimental applicability of the thermodynamic speed limits to scenarios in which systems are defined using local, rather than global, Hamiltonians. This includes the growing number of network-based models for nonequilibrium systems in which a node's dynamics are defined by its local interactions with neighboring nodes.

Let's say that each subsystem $i$ obeys SLDB. Then, $\langle\dot{\zeta}^i_{\mathcal{N}}(t)\rangle$ can be split into two contributions as follows,

$$\begin{aligned}\langle\dot{\zeta}^i_{\mathcal{N}}(t)\rangle &= \sum_{x',x} K_x^{x'}(i;t)p_{x'}(t)\ln\left[\frac{p_{x'}(t)}{p_x(t)}\right] \\ &\quad + \sum_{x',x} K_x^{x'}(i;t)p_{x'}(t)\ln\left[\frac{K_x^{x'}(i;t)}{K_{x'}^{x}(i;t)}\right]\end{aligned} \tag{S31}$$

To simplify the first sum on the RHS of Eq. (S31), using Eq. (9), we expand

$$\sum_{x',x} K_x^{x'}(i;t)p_{x'}(t)\ln\left[\frac{p_{x'}(t)}{p_x(t)}\right] \tag{S32}$$

$$= \sum_{x'_{-i}}\sum_{x_i}\sum_{x'_i\neq x_i} K_{x_i,x'_{-i}}^{x'_i,x'_{-i}}(i;t)p_{x'_i,x'_{-i}}(t)\ln\left[\frac{p_{x'_i,x'_{-i}}(t)}{p_{x_i,x'_{-i}}(t)}\right] \tag{S33}$$

$$= -\sum_{x'_{-i}}\sum_{x_i}\sum_{x'_i\neq x_i} K_{x_i,x'_{-i}}^{x'_i,x'_{-i}}(i;t)p_{x'_i,x'_{-i}}(t)\ln p_{x_i,x'_{-i}}(t) \tag{S34}$$

$$\begin{aligned}&= -\sum_{x'_{-i}}\sum_{x_i}\sum_{x'_i\neq x_i} K_{x_i,x'_{-i}}^{x'_i,x'_{-i}}(i;t)p_{x'_i,x'_{-i}}(t)\ln p_{x'_{-i}|x_i}(t) \\ &\quad - \sum_{x'_{-i}}\sum_{x_i}\sum_{x'_i\neq x_i} K_{x_i,x'_{-i}}^{x'_i,x'_{-i}}(i;t)p_{x'_i,x'_{-i}}(t)\ln p_{x_i}(t)\end{aligned} \tag{S35}$$

$$= \frac{d^i}{dt}S^{X|X_i}(t) + \frac{d}{dt}S^{X_i}(t) \tag{S36}$$

The first term on the RHS, $\frac{d^i}{dt}S^{X|X_i}(t)$, is called the the "$i$-windowed derivative of the conditional entropy". It was first defined in [12], and equals the negative of the information flow, $\langle\dot{I}^{-i\to i}\rangle$, from subsystem $i$ to the rest of the subsystems in $\mathcal{N}$. It quantifies how fluctuations in the state of subsystem $i$ affect its correlations with the rest of the system [3]. In the special case that the system is in a NESS, this term is referred to in the literature as the "learning rate" [3], i.e., the rate at which subsystem $i$ "learns" about the other subsystems $-i$. The second term on the RHS, $\frac{d}{dt}S^{X_i}(t)$, is the rate of change of the Shannon entropy of subsystem $i$, defined by the marginal distribution over only subsystem $i$'s states.

To simplify the second sum on the RHS of Eq. (S31), we note that the state transitions that contribute to $\langle\dot{\zeta}^i_{\mathcal{N}}(t)\rangle$ involve only a change in $x_i$, with the state $x'_{-i}$ held fixed. (This is because $K_x^{x'}(i;t) = 0$ if $x'_{-i}\neq x'_{-i}$.) Then, invoking SLDB, the EF associated with such a transition $x'(=x'_i,x'_{-i})\to x(=x_i,x'_{-i})$ is $Q^i_{x'\to x} = H_{x'_{r(i)}}(i;t) - H_{x_{r(i)}}(i;t)$, for some local Hamiltonians $H_{x_{r(i)}}(i;t)$. The EF rate into the subsystem $i$ is $\dot{Q}^i(t) = \sum_{x'\neq x}K_x^{x'}(i;t)p_{x'}(t)Q^i_{x'\to x}$.

Therefore, SLDB allows us to write, in a similar fashion to Eq. (5) of [9],

$$\langle\dot{\zeta}^i_{\mathcal{N}}(t)\rangle = \frac{d^i}{dt}S^{X|X_i}(t) + \frac{d}{dt}S^{X_i}(t) + \beta_i\dot{Q}^i(t) \tag{S37}$$

$$= -\langle\dot{I}^{-i\to i}\rangle + \frac{d}{dt}S^{X_i}(t) + \beta_i\dot{Q}^i(t) \tag{S38}$$

Similarly, *mutatis mutandis*, for every unit $\omega$ such that $i\in\omega$,

$$\langle\dot{\zeta}^i_{\omega}(t)\rangle = \frac{d^i}{dt}S^{X_\omega|X_i}(t) + \frac{d}{dt}S^{X_i}(t) + \beta_i\dot{Q}^i(t) \tag{S39}$$

$$= -\langle\dot{I}^{-i\to\omega\setminus i}\rangle + \frac{d}{dt}S^{X_i}(t) + \beta_i\dot{Q}^i(t) \tag{S40}$$

We see, therefore, that subsystem $i$'s contribution to the system's (or a unit's) EP rate consists of (i) the information flow between $i$ and the rest of the system (unit), (ii) the rate of change of Shannon entropy of

the marginal distribution of $i$, and (iii) the EF rate into subsystem $i$ from its reservoir(s). Eq. (S38) was also derived in [3], but without explicit use of the SLDB condition. This establishes thermodynamic consistency and experimental applicability of the quantities $\langle \dot{\zeta}^i_{\mathcal{N}}(t)\rangle$ and $\langle \dot{\zeta}^i_{\omega}(t)\rangle$.

## S5 Integral Fluctuation Theorem (IFT) on Subsystem-Indexed Contributions to the Global EP

We note that it follows immediately from the result in [10] that each of the subsystem-indexed contributions to the global (or unit-local) EP follows an IFT:

$$\forall i \in \mathcal{N},\ \omega \in \mathcal{N}^{\dagger} | i \in \omega,\ t > 0 : \langle e^{-\zeta^i_{\omega}(\tau)}\rangle = 1 \tag{S41}$$

where the trajectory-level subsystem contribution to the EP is $\zeta^i_{\omega}(\boldsymbol{x}) = -I^{\omega\setminus i \to i}(\boldsymbol{x}) + \Delta s^i(\boldsymbol{x}) + \beta_i Q^i(\boldsymbol{x})$. As usual, $\Delta s^i = p_{x_i}(t) - p_{x_i}(0)$ is the change in the trajectory-level entropy of the marginal distribution of $i$, and $Q^i$ is the total trajectory-level entropy flow into $i$ from its reservoirs (refer to the definition in [14]). $I^{\omega\setminus i\to i}(\boldsymbol{x})$ is the total information flow into subsystem $i$ from the set of subsystems $\omega \setminus i$.

More generally, we can consider a set of subsystems $A \in \omega$ which has a contribution to the EP of the unit $\omega$. Since we can validly replace $i \to A$ in all of the above definitions of thermodynamic quantities, we know

$$\forall A \in \mathcal{N},\ \omega \in \mathcal{N}^{\dagger} | A \in \omega,\ t > 0 : \langle e^{-\zeta^A_{\omega}(\tau)}\rangle = 1 \tag{S42}$$

## S6 Unit-Local Speed Limits for MPPs

In order for the global system to reach a certain distribution $p_x(\tau)$ by time $\tau$, each unit $\omega$ must have also reached the corresponding marginal distribution $p_{x_\omega}(\tau) = \sum_{x_{-\omega}} p_x(\tau)$ by time $\tau$. Therefore, by applying the SLT to each of the units in $\mathcal{N}^{**}$ we get a set of additional lower bounds on the speed of system evolution:

$$\forall\, \omega \in \mathcal{N}^{**}\ : \tau \geq \frac{\left(\mathcal{L}(p_{x_\omega}(0), p_{x_\omega}(\tau))\right)^2}{2\langle \sigma^{\omega}(\tau)\rangle \langle \mathcal{A}^{\omega}\rangle_{\tau}} \tag{S43}$$

These bounds form the set of **unit-local SLTs** for an MPP. Here, $\mathcal{L}(p_{x_\omega}(0), p_{x_\omega}(\tau)) = \sum_{x_\omega} |p_{x_\omega}(0) - p_{x_\omega}(\tau)|$ is the $\omega$-local marginal total variation distance, $\langle \mathcal{A}^{\omega}\rangle_{\tau} = \frac{1}{\tau}\int_0^{\tau} \sum_{x'_\omega \neq x_\omega} dt K^{x'_\omega}_{x_\omega}(\omega;t) p_{x'_\omega}(t)$ is the $\omega$-local time-averaged dynamical activity, and $\langle \sigma^{\omega}(\tau)\rangle = \int_0^{\tau} dt \sum_{x'_\omega, x_\omega} K^{x'_\omega}_{x_\omega}(\omega;t) p_{x'_\omega}(t) \ln\left[\frac{K^{x'_\omega}_{x_\omega}(\omega;t) p_{x'_\omega}(t)}{K^{x_\omega}_{x'_\omega}(\omega;t) p_{x_\omega}(t)}\right]$ is the $\omega$-local EP.

We note that the bound in our second main result, Eq. (19), is always at least as tight as the bound in the unit-local SLT Eq. (S43) for the unit $\omega$ because of the Cauchy-Schwartz inequality, which gives $\left(\sum_{i\in\omega} \sqrt{\langle \zeta^i_{\omega}(\tau)\rangle \langle \mathcal{A}^i\rangle_{\tau}}\right)^2 \leq \langle \sigma^{\omega}(\tau)\rangle \langle \mathcal{A}^{\omega}\rangle_{\tau}$.

We further note in Section S7 that the strongest of a generalized form of the SLT that involves a linear combination of unit-local thermodynamic properties is given by the unit-local SLT for the system's slowest-evolving unit.

## S7 Strongest Version of the SLT Involving Linear Combinations of Unit-Local Thermodynamic Properties is Given by a Unit-Local SLT

From the global and unit-local speed limits Eq. (S43), it follows immediately that we can bound the time of evolution of a system by applying the SLTs to any linear combination of units. Define $\mathcal{N}^{\dagger} = \mathcal{N}^{**} \cup \mathcal{N}$. Let $\vec{m}$ be an arbitrary, non-negative, unit-indexed vector $\vec{m} \in \{\mathbb{R}^+_0\}^{|\mathcal{N}^{\dagger}|}$. For any such $\vec{m}$, the following **generalized SLT** holds in an MPP:

$$\tau \geq \frac{\sum_{\omega\in\mathcal{N}^{\dagger}} m_{\omega} c^{\omega}(\tau)}{\sum_{\omega'\in\mathcal{N}^{\dagger}} m_{\omega'} \langle \sigma^{\omega'}\rangle} \tag{S44}$$

where, for each unit $\omega$, we have defined the function $c^{\omega}(\tau) = \frac{\left(\mathcal{L}(p_{x_\omega}(0), p_{x_\omega}(\tau))\right)^2}{2\langle \mathcal{A}^{\omega}\rangle_\tau}$. To see this, weight the unit-local SLT Eq. (S43) for each $\omega \in \mathcal{N}^\dagger$ by $m_\omega$, add these inequalities together, and rearrange into a lower bound on $\tau$. Intuitively, a specific value of $\vec{m}$ corresponds to using a particular weighting of the local thermodynamic properties of different units in bounding the speed of system evolution.

We will now use the generalized mediant inequality to derive the tightest of these bounds. It states that the weighted mediant of $n$ fractions, $\frac{a_1}{b_1}, \frac{a_2}{b_2}, \ldots, \frac{a_n}{b_n}$, with weights $w_i \geq 0$, lies between the largest and smallest values of the fractions $\frac{a_i}{b_i}$:

$$\min_i \frac{a_i}{b_i} \leq \frac{\sum_i w_i a_i}{\sum_j w_j b_j} \leq \max_i \frac{a_i}{b_i} \tag{S45}$$

Taking the $i$ as units, $w_i$ becomes $m_\omega$, each $a_i$ becomes $c^{\omega}(\tau)$, and each $b_i$ becomes $\langle \sigma^{\omega}\rangle$. It immediately follows that

$$\min_{\omega\in\mathcal{N}^\dagger} \frac{c^{\omega}(\tau)}{\langle \sigma^{\omega}\rangle} \leq \frac{\sum_{\omega\in\mathcal{N}^\dagger} m_\omega c^{\omega}(\tau)}{\sum_{\omega'\in\mathcal{N}^\dagger} m_{\omega'}\langle \sigma^{\omega'}\rangle} \leq \max_{\omega\in\mathcal{N}^\dagger} \frac{c^{\omega}(\tau)}{\langle \sigma^{\omega}\rangle} \tag{S46}$$

The tightest (loosest) bound in the set of bounds defined by Eq. (S44) is achieved when $\vec{m}$ is a Dirac-delta function over the space of units ($\mathcal{N}^\dagger$) such that the only non-zero value of $m_\omega$ is the one for the slowest-evolving (fastest-evolving) unit, i.e., the unit with the largest (smallest) value of the bound in its local SLT. Intuitively, the slowest-evolving (fastest-evolving) unit (SEU, FEU) corresponds to the unit for which the local thermodynamic and dynamical properties of its evolution are low (high) enough that in the best case scenario, out of all the units, this unit would take the most (least) time to reach its desired final distribution.

# S8 Unit-Local Speed Limits More Tightly Constrain Space of Accessible Distributions than Global Speed Limit (Shown for the Case of Two Independent Bits)

For simplicity of illustration, consider the general case of an MPP with $n$ non-overlapping units $\omega$, each with $|X_\omega| = k$ possible states. The total number of joint states is then $|X| = k^n$. All valid joint probability distributions comprise the $(k^n - 1)$-simplex, $\Delta^{k^n-1}$ (with side length $\sqrt{2}$). For our calculations we embed this simplex in $k^n$-space, where it is an $(k^n - 1)$-dimensional manifold. The global SLT, which states $\sum_x |p_x(\tau) - p_x(0)| \leq \sqrt{2\tau\langle\sigma\rangle\langle\mathcal{A}\rangle_\tau}$, restricts the space of accessible distributions to the intersection between $\Delta^{k^n-1}$ and $B_1^{k^n}(p_x(0))$. $B_1^{k^n}(p_x(0))$ is the $k^n$-cross polytope ($l_1^{k^n}$ ball) with edge length $\sqrt{2} \times \sqrt{2\tau\langle\sigma\rangle\langle\mathcal{A}\rangle_\tau}$ centered at the point on $\Delta^{k^n-1}$ that represents the initial joint distribution, $p_x(0)$.

Each unit-local SLT Eq. (S43), which states $\sum_{x_\omega} \left|p_{x_\omega}(\tau) - p_{x_\omega}(0)\right| \leq \sqrt{2\tau\langle\sigma^{\omega}\rangle\langle\mathcal{A}^{\omega}\rangle_\tau}$, further restricts this space of accessible distributions to the collection of points in $\Delta^{k^n-1}$ that are consistent with the intersection of the marginal simplex $\Delta^{k-1}$ with $B_1^k(p_{x_\omega}(0))$. $B_1^k(p_{x_\omega}(0))$ is the $k$-cross polytope with edge length $\sqrt{2} \times \sqrt{2\tau\langle\sigma^{\omega}\rangle\langle\mathcal{A}^{\omega}\rangle_\tau}$) centered at the point on the $\Delta^{k-1}$ that represents its initial marginal distribution, $p_{x_\omega}(0) = \sum_{x_{-\omega}} p_x(0)$. Similar geometric relations hold for overlapping units.

To demonstrate a calculation, we proceed by considering an MPP consisting of $n$ independent bits that don't necessarily evolve according to the same rate matrix. Thus, any bit $i$ generates an EP of $\langle\sigma^i\rangle \leq \langle\sigma\rangle$ in the interval $[0, \tau]$. Additionally, the time-averaged dynamical activity of any bit $i$ is $\langle\mathcal{A}^i\rangle_\tau \leq \langle\mathcal{A}\rangle_\tau$.

Let us consider the case of $n = 2$ independent bits, $i$ and $j$. This means that each bit comprises its own unit, which doesn't overlap with the other. For accompanying illustrations, see Fig. S1. Let's also say that the initial joint distribution is a Kronecker-delta function centered at $p_{11}$, i.e. $p_{ij}(0) : p_{00}(0) = 0, p_{01}(0) = 0, p_{10}(0) = 0, p_{11}(0) = 1$. Due to the symmetry of the problem, the following calculations hold for a delta function initial distribution centered at any one of the four joint states. All final joint distributions $p_{ij}(\tau)$ must lie on the simplex $\Delta^3$, which can be visualized as a tetrahedron. The total volume $V_t$ of this space of distributions is 1/3 (remember that a probability simplex has side length $\sqrt{2}$).

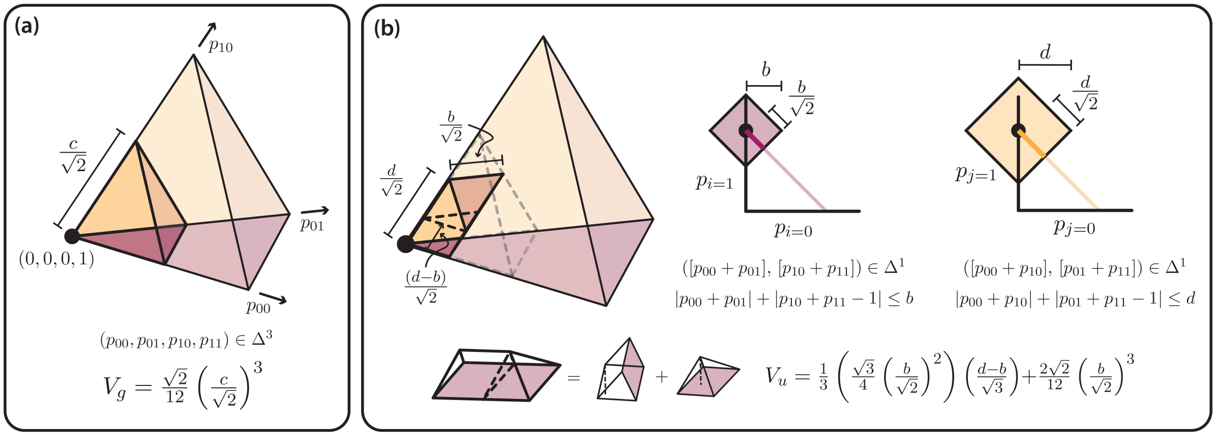


Figure S1: For two independent bits, the set of unit-local SLTs more tightly restricts the space of accessible final joint distributions than does the global SLT. Geometrical representations and calculations of the space of accessible distributions as restricted by (a) the global SLT alone and by (b) the set of unit-local SLTs are shown for the case of two independently evolving bits. In both panels, the large tetrahedron represents the 3-simplex that constrains all probability distributions with 4 possible states, and the highlighted convex hull within its interior represents the space of joint distributions accessible by time $\tau$. In (b) right, the 2D graphs show the space of accessible marginal distributions for each individual bit (shaded squares), as given by the unit-local SLTs. In (b) left, the joint distributions that are consistent with these marginal distributions form the highlighted convex hull. The dotted grey lines represent the convex hull of the space of accessible joint distributions as constricted by the global SLT, and are provided for visual comparison to the space consistent with the unit-local SLTs.

We can write out the global SLT as:

$$\sqrt{2\tau\langle\sigma\rangle\langle\mathcal{A}\rangle_\tau} = c \geq |p_{00}(\tau)| + |p_{01}(\tau)| + |p_{10}(\tau)| + |p_{11}(\tau) - 1| \tag{S47}$$

The RHS is representable by the $B_1^4(p_{ij}(0))$, which is a 16-cell centered at one corner of $\Delta^3$. The intersection of this off-centered $l_1^4$ ball with $\Delta^3$ is $\Delta_g^3$, a scaled-down version of the 3-simplex with side length $\frac{c}{\sqrt{2}}$, and this is the set of accessible distributions as restricted by the global SLT alone. The volume $V_g$ of (the convex hull of) this set of points reachable in time $\tau$ by the global SLT is the volume of a tetrahedron of side length $\frac{c}{\sqrt{2}}$. Thus $V_g = c^3/24$. Therefore, the fraction of distributions reachable in time $\tau$ by the global SLT is $f_g = V_g/V_t = c^3/8$. Note, by extension, that for any system with a total of $|X|$ states and delta-function initial distribution, the fraction of distributions reachable in time $\tau$ as constrained by the global SLT is $(\frac{c}{2})^{|X|-1}$.

Now we consider the restrictions placed by the unit-local SLTs for each bit. Since the bits are independent, it must hold that $\langle\sigma\rangle = \langle\sigma^i\rangle + \langle\sigma^j\rangle - \langle\Delta\mathcal{I}^{\mathcal{N}^*}\rangle$ (where $\langle\Delta\mathcal{I}^{\mathcal{N}^*}\rangle$ is the change in inclusion-exclusion information defined in [12]) and $\langle\mathcal{A}\rangle_\tau = \langle\mathcal{A}^i\rangle_\tau + \langle\mathcal{A}^j\rangle_\tau$. We write out the unit-local SLTs as:

$$\sqrt{2\tau\langle\sigma^i\rangle\langle\mathcal{A}^i\rangle_\tau} = b \geq |p_{00}(\tau) + p_{01}(\tau)| + |p_{10}(\tau) + p_{11}(\tau) - 1| \tag{S48}$$

$$\sqrt{2\tau\langle\sigma^j\rangle\langle\mathcal{A}^j\rangle_\tau} = d \geq |p_{00}(\tau) + p_{10}(\tau)| + |p_{01}(\tau) + p_{11}(\tau) - 1| \tag{S49}$$

where, without loss of generality, we set $b \leq d$. Using these restrictions, we can draw, as shown in Fig. S1, the convex hull of the set of points reachable in time $\tau$ by the set of these two local SLTs. To obtain this convex hull, simply note that $p_{01}$ and $p_{10}$ can increase together by $\frac{b}{\sqrt{2}}$ and $\frac{d}{\sqrt{2}}$, respectively, but that for any

other pair of joint probabilities, the *sum* of their probabilities (i.e. $p_{00} + p_{10}$ or $p_{00} + p_{01}$) can at maximum change by $\min[\frac{b}{\sqrt{2}}, \frac{d}{\sqrt{2}}] = \frac{b}{\sqrt{2}}$. The volume $V_u$ of this convex hull, as shown in Fig. S1b, is $\frac{b^2(d-b)}{8} + \frac{b^3}{12}$. Therefore, the fraction of distributions reachable in time $\tau$ by the global SLT is $f_u = \frac{3b^2(d-b)}{8} + \frac{b^3}{4}$. Therefore, for two identical but independently-evolving bits,

$$\frac{f_u}{f_g} = \frac{3b^2(d-b) + 2b^3}{c^3} \tag{S50}$$

Note that in the case that $b = d = \frac{c}{2}$, this reduces to $\frac{1}{4}$. Also note that for the case of $n = 1$ bit, or for a set of fully connected bits (where each bit interacts with all other bits), the only unit is the global system itself, and thus there exist no local SLTs apart from the global SLT. Therefore, in this case, $\frac{f_u = f_g}{f_g} = 1$.

We suspect that it is true in general (for any type of unit structure and for any initial distribution) that the unit-local SLTs combined with the global SLT more tightly restrict the space of accessible final distributions than does the global SLT alone. We posit this is because the unit-local SLTs, since they involve marginal distributions, provide multiple constraints on the same joint probabilities. Note that if all of the transitions in a system occur in a single unit, the unit-local SLTs reduce to the global SLT and no additional constraints are possible. We also suspect that the MPP SLTs we show in the main text (and derived in Sections S1 and S2) taken together would more tightly constrain the space of accessible final distributions than the global SLTs, and potentially even the unit-local SLTs taken together. We leave these investigations for future work.

## S9 Maximum and Minimum Speeds for Bayes' Nets

We can run an MPP as a Bayes' Net (BN) [13]. This means that state transitions are no longer stochastically timed, but occur according to a global, synchronous clock. Therefore, for the results in this section, we are concerned with discrete-time thermodynamics instead of continuous-time dynamics as we were for the more general case of MPPs. We emphasize that although a BN is a special case of an MPP, the SLTs for MPPs do not reduce simply to the SLTs for BNs. We derive these results from relations specific to BNs (and which don't apply to MPPs). We therefore introduce these BN-specific relations here.

In a BN, For any times $t$, $t' > t$, the joint distribution at $t'$ is

$$\begin{aligned} p(x_1^{t'}, x_2^{t'}, \ldots) = \\ \sum_{x_1^t, x_2^t, \ldots} p(x_1^{t'}, x_2^{t'}, \ldots | x_1^t, x_2^t, \ldots) p(x_1^t, x_2^t, \ldots) \end{aligned} \tag{S51}$$

Typically, there are conditional independencies in how each of the subsystems evolve. In general, this means that $p(x_1^{t'}, x_2^{t'}, \ldots | x_1^t, x_2^t, \ldots)$ can be decomposed into a product of conditional distributions, each of which captures one of those conditional independencies. If we consider the example in Fig. **??** and take instead as subsystems $A$, $B$, and $C$, retaining the same dependency constraints, and set $x_B^{t'} = x_B^t$ with probability 1, then

$$\begin{aligned} p(x_A^{t'}, x_B^{t'}, x_C^{t'} | x_A^t, x_B^t, x_C^t) = \\ p(x_A^{t'} | x_A^t, x_B^t) p(x_C^{t'} | x_B^t, x_C^t) \delta(x_B^{t'}, x_B^t). \end{aligned} \tag{S52}$$

These conditional (in)dependencies can be represented as a directed acyclic graph (DAG), as shown in Fig. S2. This representation of a distribution is an example of a Bayes' net. BNs can be generalized to represent the dynamics over an arbitrary number of subsystems. In addition, they can represent dynamics over an arbitrary number of times, not just the two times illustrated in Fig. S2(a), simply by adding more layers to the DAG.

Following the convention in [13, 5], we restrict attention to BNs where only one node's conditional distribution is implemented at a time. This means the evolution of any node $v$ in the BN occurs in a solitary process, where the evolving system $a$ is the union of the subsystem corresponding to $v$ and the subsystems

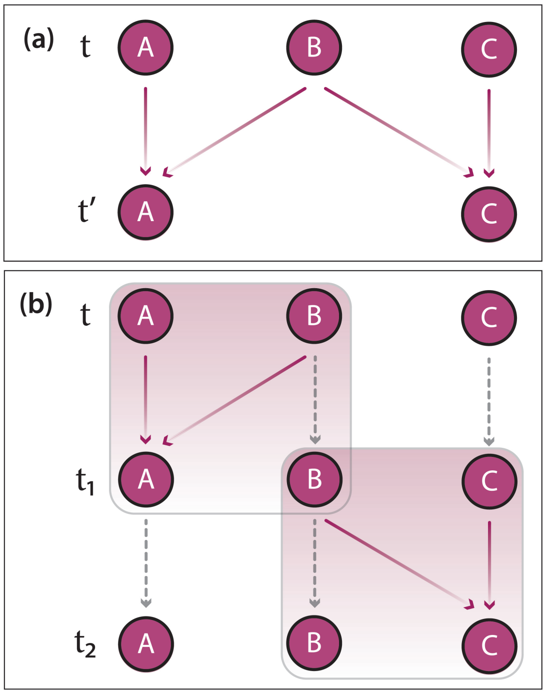


Figure S2: (a) An example BN showing the conditional independencies between subsystems $A$, $B$, and $C$. The top three nodes are the root nodes of the DAG, representing the time-$t$ states of the three subsystems. The bottom nodes are the leaf nodes, representing the time-$t'$ states of two of the subsystems. (Subsystem B does not evolve, so we dispose of its leaf node.) The directed edges into the bottom-left leaf node indicate that $x_A^{t'}$ depends only on $x_A^t$ and $x_B^t$, the two parents of that node. Similarly, the edges into the bottom-right leaf node indicate that $x_C^{t'}$ depends only on $x_B^t$ and $x_C^t$, the two parents of that node. (b) An example of running the same BN as a sequence of solitary processes. Dashed gray arrows indicate the identity map. In the first solitary process, the evolving system consists of subsystems $A$ and $B$, while in the second solitary process it consists of $B$ and $C$.

corresponding to the parents of $v$. For a solitary process occurring over the time interval $[0, \tau]$, the local EP of the evolving system $a$ along a trajectory $\boldsymbol{x}$ is

$$\sigma_a(\boldsymbol{x}, p_a^0, p_a^\tau) := \left(\ln[p_a^0(\boldsymbol{x}_a^0)] - \ln[p_a^\tau(\boldsymbol{x}_a^\tau)]\right) - Q_1(\boldsymbol{x}_a) \tag{S53}$$

$Q(\boldsymbol{x})$ is the entropy flow (EF) from the heat bath into the joint system during the process. For a solitary process, $Q(\boldsymbol{x}) = Q_1(\boldsymbol{x}_a)$ for some function $Q_1$. The evolving system of a solitary process is called a solitary system, and the local EP of a solitary process is only a function of $\boldsymbol{x}_a$. The global EP generated by the evolving system $a$ and the fixed system $b$ is

$$\sigma(\boldsymbol{x}, p^0, p^\tau) = \left(\ln[p^0(\boldsymbol{x}^0)] - \ln[p^\tau(\boldsymbol{x}^\tau)]\right) - Q(\boldsymbol{x}) \tag{S54}$$

$$= \sigma_a(\boldsymbol{x}, p_a^0, p_a^\tau) - \Delta I_{p^0,p^\tau}(\boldsymbol{x}_a;\boldsymbol{x}_b) \tag{S55}$$

where $\Delta I_{p^0,p^\tau}(\boldsymbol{x}_a;\boldsymbol{x}_b)$ is the difference between the ending and starting (stochastic) mutual information between the evolving and the fixed systems.

We write the set of nodes in a BN as $V$, and label them with successive integers. In general, more than one $v \in V$ might refer to evolution of the same subsystem, just at different times. In light of the fact that the evolving system in each solitary process will be the union of a node and its parents, for any $V' \subset V$ we define $[V'] := V' \cup pa(V') := \cup_{v \in V'} v \cup pa(v)$, where $pa(v)$ indicates the parents of node $v$. In addition, for any subset $V' \subset V$, we define $-V' = V \setminus V'$. We write the distribution over all subsystems after the

process implementing node $v$ has run as $p^{t_v}$, and unless indicated otherwise, assume that it runs in the time interval $[t_{v-1}, t_v]$. The root nodes are jointly sampled at $t = 0$ according to distribution $p^0(x)$, and the BN is allowed to run through all its nodes, resulting in full trajectory $\boldsymbol{x}$. For any $v \in V$, we write the segment of $\boldsymbol{x}$ corresponding to the time interval when node $v$ runs as $\boldsymbol{x}^v$, reserving superscripts for time slices and subscripts for specification of particular subsystems. As an example of this notation, $\boldsymbol{x}_{[v]}$ is the full trajectory of the components of $\boldsymbol{x}$ specified by $[v]$, while $\boldsymbol{x}^v_{[v]}$ is the segment of that trajectory in the time interval $[t_{v-1}, t_v]$.

Let $\pi = \{\pi_v(x_v|x_{pa(v)})\}$ indicate the set of the conditional distributions at the nodes of the BN. We write the local EP generated in the solitary process associated with running node $v$ as $\sigma_{[v]}$. Since EP is cumulative over time, by repeated application of Eq. (S55), once for each node in the BN, we see that the global EP incurred by running all nodes in the BN if the joint system follows trajectory $\boldsymbol{x}$ is

$$\begin{aligned} \sigma(\boldsymbol{x}, \pi, p^0) = \sum_{v=1}^{|V|} \Big[ &\sigma_{[v]}(\boldsymbol{x}^v_{[v]}, \pi_v, p^{v-1}) \\ &+ \Big( I_{p^{v-1}}(\boldsymbol{x}^{v-1}_{[v]}; \boldsymbol{x}^{v-1}_{-[v]}) - I_{p^v}(\boldsymbol{x}^v_{[v]}; \boldsymbol{x}^v_{-[v]}) \Big) \Big] \\ := \sum_{v \in V} \Big( &\sigma_{[v]}(\boldsymbol{x}) - \Delta I^v(\boldsymbol{x}) \Big) \end{aligned} \tag{S56}$$

where $\Delta I^v(\boldsymbol{x})$ is the change in (stochastic) multi-information between $[v]$ and $-[v]$. Taking the ensemble average over all trajectories $\boldsymbol{x}$, we arrive at the decomposition of the global EP in a BN,

$$\langle \sigma \rangle := \sum_{v \in V} \Big( \langle \sigma_{[v]} \rangle - \langle \Delta I^v \rangle \Big) \tag{S57}$$

We define the local dynamical activity of running the node $v$ of a BN,

$$\mathcal{A}^v_{[v]} = \sum_{x'_{[v]} \neq x_{[v]}} \sum_{i \in [v]} K^{x'_{[v]}}_{x_{[v]}}(i) p_{x'_{[v]}}(t_{v-1}), \tag{S58}$$

where $t_{v-1} = \sum_{v'=1}^{v-1} \tau_{v'}$, $t_v = t_{v-1} + \tau_v$, $x'_{[v]} = x_{[v]}(t_{v-1})$, $x_{[v]} = x_{[v]}(t_v)$, and we drop the time dependence of the rate matrix elements $K^{x'_{[v]}}_{x_{[v]}}(i)$ , because they don't change while node $v$ runs. The global and local dynamical activities are related as

$$\langle \mathcal{A} \rangle = \sum_v \langle \mathcal{A}^v_{[v]} \rangle_{\tau_v}. \tag{S59}$$

## S9.1 Speed Limits for Bayes' Net Evolution

We can plug in lower bounds analogous to the unit-local SLT for each local EP $\langle \sigma_{[v]} \rangle$ into Eq. (S57) to obtain a new SLT applicable to a BN (this follows from Eq. (S56)):

$$\langle \sigma \rangle \geq \sum_{v \in V} \left( \frac{\Big( \mathcal{L}_{[v]}(p^{t_{v-1}}, p^{t_v}) \Big)^2}{2\tau_v \langle \mathcal{A}^v_{[v]} \rangle_{\tau_v}} - \langle \Delta I^v \rangle \right) \tag{S60}$$

where $\mathcal{L}_{[v]}(p^{t_{v-1}}, p^{t_v})$ is the total variation distance in the joint distribution and $\langle \mathcal{A}^v_{[v]} \rangle_{\tau_v}$ is the time-averaged dynamical activity produced due to running node $v$, which occurs over a span of time $\tau_v = t_v - t_{v-1}$. Eq. (S60)'s lower bound on global EP is different from that obtained by treating the process as the evolution of a single physical system $\langle \sigma \rangle \geq \Big( \mathcal{L}(p^0, p^\tau) \Big)^2 / (2\tau \langle \mathcal{A} \rangle_\tau)$, where $\mathcal{L}(p^0, p^\tau)$ is the total variation distance of the system distribution and $\langle \mathcal{A} \rangle_\tau$ is the time-averaged dynamical activity produced incurred by running the entire BN during the time interval $[0, \tau]$.

For a given global EP, Eq. (S60) serves as a trade-off between changing the speed, inverse activity, and total variation distance of one step in the process (e.g. that in which node $v$ runs) and changing those of

other steps (e.g. in which other nodes $v' \neq v$ run). We can see that slowing down any particular node in the BN could potentially give a smaller lower bound on EP. Therefore, one can exploit Eq. (S60) to identify the thermodynamically costlier nodes, i.e., those with the largest value of inverse activity-weighted total variation distance $\left(\mathcal{L}_{[v]}(p^{t_{v-1}}, p^{t_v})\right)^2 / \langle \mathcal{A}^v_{[v]} \rangle_{\tau_v}$. Slowing down these particular nodes provides the most effective way to try to lower the dissipative cost of running a BN while making the fewest possible changes to the process. As a result, Eq. (S60) offers fine-grained control over a BN. In the example of a digital circuit, this translates to knowing which gates, if slowed down enough, could drastically reduce the circuit's dissipative cost. Finally, this result also shows the role of the multi-information in connecting the local run-time of a single node in the BN to the total EP of the entire BN.

We can also derive a bound for the time $\tau$ of running the entire BN. We first rearrange the speed limit for each local EP to get a local speed limit for each step in the process of running the BN:

$$\tau_v \geq \frac{\left(\mathcal{L}_{[v]}(p^{t_{v-1}}, p^{t_v})\right)^2}{2\langle \sigma_{[v]} \rangle \langle \mathcal{A}^v_{[v]} \rangle_{\tau_v}} \tag{S61}$$

Upon summing this over all steps of the BN, we obtain a system-wide speed limit:

$$\tau = \sum_v \tau_v \geq \sum_v \frac{\left(\mathcal{L}_{[v]}(p^{t_{v-1}}, p^{t_v})\right)^2}{2\langle \sigma_{[v]} \rangle \langle \mathcal{A}^v_{[v]} \rangle_{\tau_v}} \tag{S62}$$

which is different from the speed limit obtained by treating the process as the evolution of a single physical system: $\tau \geq \left(\mathcal{L}(p^0, p^\tau)\right)^2 / (2\langle \sigma \rangle \langle \mathcal{A} \rangle_\tau)$. For a given desired speed of evolution of the entire system, Eq. (S62) serves as a trade-off between the changing the local thermodynamic quantities of one step in the process (e.g. that in which node $v$ runs) versus changing those of other steps (e.g. in which other nodes $v' \neq v$ run).

Importantly, we remark that in the special case that the system begins and ends in the same non-equilibrium steady state (NESS) but can stray away from the NESS during the system evolution, the global SLTs applied to BNs provide lower bounds of zero. However, our results, Eqs. (S60) and (S62), provide strictly positive lower bounds.

## S9.2 Minimum Speeds of Bayes' Net Evolution

We now derive a minimum speed for the evolution of a BN. We start by noting that in each step of running a BN, the local EP $\langle \sigma_{[v]} \rangle$ obeys all the regular TURs. We can rearrange the thermodynamic uncertainty relation (TUR) for arbitrary initial states, derived in [6], to obtain a lower bound on the speed of evolution of for each step (i.e. running of a node $v$ of the BN)

$$\tau_v \leq \sqrt{\frac{\langle \sigma_{[v]} \rangle \mathrm{Var}(J_{[v]})}{2\langle j^{\tau_v}_{[v]} \rangle}} \tag{S63}$$

Upon summing this relation across all steps, we obtain a system-wide minimum speed (or maximum time) required to evolve the BN according to some set of instantaneous currents $\{\langle j^{\tau_v}_{[v]} \rangle\}$ and with a variance in the accumulated current $\mathrm{Var}(J_{[v]})$:

$$\tau = \sum_v \tau_v \leq \sum_v \sqrt{\frac{\langle \sigma_{[v]} \rangle \mathrm{Var}(J_{[v]})}{2\langle j^{\tau_v}_{[v]} \rangle}} \tag{S64}$$

where for a local current $J_{[v]}$ produced by running a node $v$, $\mathrm{Var}(J_{[v]})$ is a measure of the bulk local current fluctuations and $\langle j^{\tau_v}_{[v]} \rangle$ is the ensemble-average local instantaneous current observed right when node $v$ has finished running. This minimum speed (Eq. (S64)) is different from that obtained by treating the BN as a single, undecomposed physical system: $\tau \leq \sqrt{(\langle \sigma \rangle \mathrm{Var}(J))/(2\langle j^\tau \rangle)}$, where for a global current $J$ produced by running the entire BN, $\mathrm{Var}(J)$ is a measure of the bulk global current fluctuations and $\langle j^\tau \rangle$ is the instantaneous final current observed after running the entire BN.

For an engineer with a maximum allowable time of BN evolution, Eq. (S64) can be interpreted as a trade-off between changing the precisions of local bulk currents, the local EPs, and the local instantaneous currents of each step in the process (i.e. running node $v$) versus changing those quantities for another step (i.e. running node $v' \neq v$).

## S10 Lower Bounds on the Difference between the EP Rate and the Rate at which One Unit Learns about Another Based on Counterfactual Thermodynamic Quantities

Here we utilize the decomposition of the global expected EP rate as derived in [12]:

$$\begin{aligned}\langle \dot{\sigma}(t)\rangle = \langle \dot{\sigma}^{\phi}(t)\rangle + \langle \dot{\sigma}_{K(\omega\setminus\phi;t);\omega}(t)\rangle + \langle \dot{\sigma}_{K(\mathcal{N}\setminus\omega;t)}(t)\rangle \\ + \frac{d^{\phi}}{dt} S^{X_\omega|X_\phi}(t) + \frac{d^{\omega}}{dt} S^{X|X_\omega}(t)\end{aligned} \tag{S65}$$

where $\omega$ and $\phi \subset \omega$ are both units under $K_x^{x'}(t)$. This equation applies to the example MPP in Fig. 1.

The first term on the RHS, $\langle \dot{\sigma}^{\phi}(t)\rangle$, is the local expected EP rate of the unit $\phi$ at time $t$. The second term, $\langle \dot{\sigma}_{K(\omega\setminus\phi;t);\omega}(t)\rangle$ is the expected EP rate of the unit $\omega$ at time $t$ if at that instant it were to evolve for an infinitesimal time $\delta t$ under the counterfactual rate matrix $K(\omega\setminus\phi;t)$. Similarly, the third term, $\langle \dot{\sigma}_{K(\mathcal{N}\setminus\omega;t)}(t)\rangle$ is the expected EP rate of the entire system at time $t$ if at that instant it were to evolve for an infinitesimal time $\delta t$ under the counterfactual rate matrix $K(\mathcal{N}\setminus\omega;t)$. The counterfactual rate matrix $K(A;t)$ indicates the rate matrix if at time $t$ only the subsystems in $A$ are allowed to change state, and the states of the remaining subsystems in the system are held fixed. In a physical system, this corresponds to the counterfactual case of removing the reservoirs coupled to the subsystems in $\mathcal{N}\setminus A$ at time $t$.

The fourth term on the RHS is the windowed $\phi$-derivative of the conditional entropy in $X_\omega$ given $X_\phi$. It is a measure of how quickly the statistical coupling between $X_\omega$ and $X_{\omega\setminus\phi}$ changes at time $t$, if rather than evolving under the actual rate matrix, the system were to evolve under a counterfactual rate matrix $K(\phi;t)$ in which $x_{\omega\setminus\phi}$ is not allowed to change. Similarly, the fifth term is the windowed $\omega$-derivative of the conditional entropy in $X$ given $X_\omega$. We note that the general quantity $\frac{d^A}{dt} S^{X|X_A}(t)$ is the derivative of the negative mutual information between $X_A$ and $X_{-A}$ under the counterfactual rate matrix $K(A;t)$, because $S^{X_{-A}}(t)$ doesn't change under that counterfactual rate matrix. In the special case of two subsystems, both leading each other, with $A$ as one of those subsystems, $\frac{d^A}{dt} S^{X|X_A}(t)$ is the same as the "information flow", termed the learning rate, analyzed in [4, 1]. See Eq. 4 in [3] for a generalization of information flows to multiple subsystems that is similar to the general expression $\frac{d^A}{dt} S^{X|X_A}(t)$. We can therefore identify $\frac{d^\phi}{dt} S^{X_\omega|X_\phi}(t)$ as the rate at which unit $\phi$ learns about the set of subsystems, $\omega\setminus\phi$, in unit $\omega$ but not in $\phi$.

To proceed, we will now derive relations to instantaneous changes in distributions. We begin with the definition for a generalized counterfactual EP rate:

$$\begin{aligned}&\langle \dot{\sigma}_{K(A;t);B}(t)\rangle = \\ &\qquad \sum_{x_B, x'_B} K_{x_B}^{x'_B}(A;t) p_{x'_B}(t) \ln \frac{K_{x_B}^{x'_B}(A;t) p_{x'_B}(t)}{K_{x'_B}^{x_B}(A;t) p_{x_B}(t)},\end{aligned} \tag{S66}$$

where $A \subseteq B \subseteq \mathcal{N}$, and $B$ is a unit, but $A$ is not necessarily a unit. $K_{x_B}^{x'_B}(A;t)p_{x'_B}(t)$ is the infinitesmal probability flow from $x'_B \to x_B$ in the distribution $p_{X_B}$ if at that instant in time, $p_{X_B}$ were to evolve under $K(A;t)$ instead of $K(B;t)$. $K_{x'_B}^{x_B}(A;t)p_{x_B}(t)$ is the infinitesmal probability flow from $x_B \to x'_B$ in that same situation. These quantities can also be viewed as the frequency of jumps between those states $x'_B$ and $x_B$ *if* the entire distribution over $X_B$ were to evolve under the counterfactual rate matrix at that instant in time. This means that these quantities are related to the instantaneous counterfactual dynamical activity,

$$\mathcal{A}^{B;K(A;t)}(t) := \sum_{x'_B \neq x_B} K_{x_B}^{x'_B}(A;t) p_{x'_B}(t). \tag{S67}$$

Following the analysis in [11], we define $\pi_{x_B}^{x'_B}$ as the forward transition from $x'_B \to x_B (\neq x'_B)$ and introduce a probability distribution for the forward transition under the counterfactual rate matrix:

$$\overrightarrow{P}_{K(A;t)}(\pi_{x_B}^{x'_B})(t) := (\mathcal{A}^{B;K(A;t)}(t))^{-1}(K_{x_B}^{x'_B}(A;t)p_{x'_B}(t)). \tag{S68}$$

Similarly, the probability distribution of the backward transition $\pi_{x'_B}^{x_B}$ from $x_B \to x'_B$ under the counterfactual rate matrix is

$$\overleftarrow{P}_{K(A;t)}(\pi_{x'_B}^{x_B})(t) := (\mathcal{A}^{B;K(A;t)}(t))^{-1}(K_{x'_B}^{x_B}(A;t)p_{x_B}(t)). \tag{S69}$$

The counterfactual EP rate can thus be rewritten as

$$\begin{aligned}&\langle \dot{\sigma}_{K(A;t);B}(t)\rangle = \\ &\quad \mathcal{A}^{B;K(A;t)}(t) * D[\overrightarrow{P}_{K(A;t)}(\pi_{x_B}^{x'_B})(t) \| \overleftarrow{P}_{K(A;t)}(\pi_{x'_B}^{x_B})(t)].\end{aligned} \tag{S70}$$

We can then apply the same analysis as in Eqs. (16) - (19) of [11] to arrive at

$$\sqrt{2\mathcal{A}^{B;K(A;t)}(t)\langle \dot{\sigma}_{K(A;t);B}(t)\rangle} \geq \sum_{x_B}\left|\frac{d^{K(A;t)}}{dt}p_{x_B}(t)\right|, \tag{S71}$$

where $\frac{d^{K(A;t)}}{dt}p_{x_B}(t)$ is the instantaneous counterfactual change in the probability $p_{x_B}(t)$ if at that moment the distribution $p^{X_B}$ evolved according to the counterfactual rate matrix $K(A;t)$ instead of the rate matrix $K(B;t)$ (under which it will actually evolve). In Fig. S3, this counterfactual infinitesemal change is represented by the dotted lines, whereas the actual evolution of the probability distributions $\dot{p}_{x_B}(t)$ and $\dot{p}_{x_B}^{A}(t)$ are represented by the solid lines.

We also define the following relation for the derivative of the total variation distance of a distribution $p_{x_B}$ under a counterfactual rate matrix $K(A;t)$

$$\begin{aligned}&\lim_{\delta t \to 0} \frac{\delta \mathcal{L}^{B;K(A;t)}(p_{x_B}(t))}{\delta t} = \\ &\quad \lim_{\delta t \to 0} \frac{\sum_{x_B}\left|p_{x_B}(t) - p_{x_B}^{K(A;t)}(t+\delta t)\right|}{\delta t}\end{aligned} \tag{S72}$$

$$\dot{\mathcal{L}}^{B;K(A;t)}(p_{x_B}(t)) = \sum_{x_B}\left|\frac{d^{K(A;t)}}{dt}p_{x_B}(t)\right| \tag{S73}$$

where $\frac{d^{K(A;t)}}{dt}p_{x_B}(t)$ is the distribution at time $t+\delta t$ if $p_{x_B}(t)$ were evolved using the rate matrix $K^B(A;t)$ for a time $\delta t$.

We can then arrive at the desired lower bound on a generalized counterfactual EP rate:

$$\begin{aligned}&\langle \dot{\sigma}_{K(A;t);B}(t)\rangle \geq \\ &\quad \frac{\left(\sum_{x_B}\left|\frac{d^{K(A;t)}}{dt}p_{x_B}(t)\right|\right)^2}{2\mathcal{A}^{B;K(A;t)}(t)} = \frac{\left(\dot{\mathcal{L}}^{K(A;t)}(p_{x_B}(t))\right)^2}{2\mathcal{A}^{B;K(A;t)}(t)},\end{aligned} \tag{S74}$$

where $\dot{\mathcal{L}}^{K(A;t)}(p_{x_B}(t))$ is the instantaneous rate of change of the distribution $p_{X_B}$ and $\mathcal{A}^{B;K(A;t)}(t)$ is the instantaneous dynamical activity in unit $B$ if, at that time $t$, $p_{X_B}$ were to evolve under the counterfactual rate matrix $K(A;t)$. Eq. (S74) provides an upper bound on the (inverse activity-weighted) instantaneous change in the probability distribution over $X_B$ if the subsystems in $B \setminus A$ were not allowed to change state. Note that it would be mathematically incorrect to integrate these results over time to obtain speed limits for system evolution. The trouble arises from trying to integrate the quantities in Eq. (S71) over time, since such a time integral would equate to path-integrating over the disjointed dotted paths in Fig. S3. For example, integrating expected counterfactual EP rate $\langle \dot{\sigma}_{K(A;t);B}(t)\rangle$ over time to get $\langle \sigma_{K(A;t);B}(t)\rangle$, the "total EP if at each

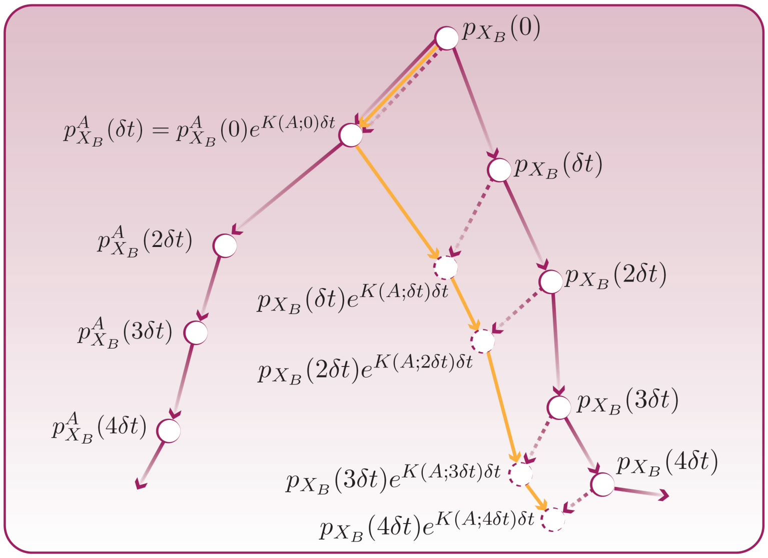


Figure S3: An illustration of the mathematical complication involved in calculating the time-integral of the instantaneous counterfactual EP rate. The white circular dots represent instantaneous probability distributions. The arrows represent the evolution of probability distributions for infinitesimal times. The leftward path of solid magenta arrows represents the evolution of the probability distribution over unit $B$ under a rate matrix $K(A;t)$ which at every time $t$ only allows the subsystems in $A \subset B$ to change state. The rightward path of solid magenta arrows represents the evolution of the probability distribution over unit $B$ under the actual rate matrix $K(B;t)$. Each dotted magenta arrow represents the evolution of the actual probability distribution $p_{x_B}(t)$ if at time $t$ it were to evolve for an infinitesimal time period $\delta t$ under the counterfactual rate matrix $K(A;t)$. This means that the states of subsystems in $B \backslash A$ would be held fixed for that infinitesimal time period $\delta t$. Since the set of dotted arrows do not provide a continuous path integral over which to integrate thermodynamic quantities, such time integrals cannot be consistently evaluated *unless* it would be mathematically equivalent to integrate instead over the yellow path. The yellow path represents an experimentally inaccessible evolution between disjoint probability distributions.

instantaneous point in time the probability distribution *were to* evolve under a counterfactual rate matrix" wouldn't make sense *unless* it is acceptable to equate such a time integral to a path integral over the yellow path in Fig. S3.

We also note that in Appendix C of [12], it is shown that the fourth and fifth terms on the RHS of Eq. (S65) are non-negative. Using the non-negativity of the fourth term and plugging in relevant versions of Eq. (S74), we obtain the following result. For any time $t$,

$$\begin{aligned}&\langle \dot{\sigma}(t) \rangle - \frac{d^\omega}{dt} S^{X|X_\omega}(t) \geq \\ &\frac{\left(\dot{\mathcal{L}}(p_{x_\phi}(t))\right)^2}{2\mathcal{A}^\phi(t)} + \frac{\left(\dot{\mathcal{L}}^{K(\omega\backslash\phi;t)}(p_{x_\omega}(t))\right)^2}{2\mathcal{A}^{\omega;K(\omega\backslash\phi;t)}(t)} + \frac{\left(\dot{\mathcal{L}}^{K(\mathcal{N}\backslash\omega;t)}(p_x(t))\right)^2}{2\mathcal{A}^{\mathcal{N};K(\mathcal{N}\backslash\omega;t)}(t)}\end{aligned} \tag{S75}$$

This inequality provides, for any time $t$, a lower bound on how much greater the global EP rate must be than the rate at which the subsystems in $\omega$ learns about the subsystems in $-\omega$ (the $\omega - \mathcal{N}$ learning rate). This bound involves counterfactual instantaneous dynamical activities and counterfactual instantaneous total variation distances of the probability distributions over units $\phi \subset \omega$, $\omega$, and $\mathcal{N}$. These quantities are either evaluated under the actual rate matrix or under an instantaneous (i.e. evaluated at time $t$) counterfactual rate matrix. This inequality can also be interpreted as an upper bound on the thermodynamically allowable instantaneous (inverse activity-weighted) change in the distributions of these units under actual or counterfactual rate matrices.

If we also incorporate the non-negativity of the fifth term on the RHS of Eq. (S65), we obtain

$$\begin{aligned}\langle\dot{\sigma}(t)\rangle \geq \frac{\left(\dot{\mathcal{L}}(p_{x_\phi}(t))\right)^2}{2\mathcal{A}^{\phi}(t)} + \frac{\left(\dot{\mathcal{L}}^{K(\omega\setminus\phi;t)}(p_{x_\omega}(t))\right)^2}{2\mathcal{A}^{\omega;K(\omega\setminus\phi;t)}(t)} \\ + \frac{\left(\dot{\mathcal{L}}^{K(\mathcal{N}\setminus\omega;t)}(p_x(t))\right)^2}{2\mathcal{A}^{\mathcal{N};K(\mathcal{N}\setminus\omega;t)}(t)}\end{aligned} \tag{S76}$$

Eq. (S76) states that, for the evolution of $\phi$ during $[0,\tau]$, there is a greater entropic cost than would be expected by the classical speed limit derived from properties only related to $\phi$. This is due to the way in which the subsystems in $\phi$ interact with other subsystems within a larger dependency structure. The classical speed limit indirectly (i.e., if the last application of the Cauchy-Schwartz inequality to the time integrals in its derivation is omitted) gives a lower bound on the EP rate for unit $\phi$ that equals the first term on the RHS of Eq. (S76). When considering the composite system within which $\phi$ resides, however, we realize that there is an increased instantaneous minimal thermodynamic cost (in terms of EP rate) that must be paid. This increased cost is equal to the second and third terms on the RHS. The second term equals the minimal cost in EP rate of evolving unit $\omega$, of which $\phi$ is a subset, during $[0,\tau]$ if the subsystems in $\phi$ remain fixed. The third term equals the minimal cost in EP rate of evolving the global system $\mathcal{N}$, of which $\omega$ is a subset, during $[0,\tau]$ if the subsystems in $\omega$ remain in a fixed state. Since these two terms are positive, Eq. (S76) thus provides a lower bound on the instantaneous global EP rate that is tighter than the lower bound obtained from the classical speed limit derived from the dynamics of one unit. Thus, we show that knowing the details of the larger dependency structure provides a stronger lower bound on the global EP rate.

Instead of replacing the local EP rate of $\phi$ with its lower bound, we could also keep the $\phi$-local EP rate in Eq. (S76) and rearrange to obtain

$$\begin{aligned}\langle\dot{\sigma}(t)\rangle - \langle\dot{\sigma}^{\phi}(t)\rangle \geq \\ \frac{\left(\dot{\mathcal{L}}^{K(\omega\setminus\phi;t)}(p_{x_\omega}(t))\right)^2}{2\mathcal{A}^{\omega;K(\omega\setminus\phi;t)}(t)} + \frac{\left(\dot{\mathcal{L}}^{K(\mathcal{N}\setminus\omega;t)}(p_x(t))\right)^2}{2\mathcal{A}^{\mathcal{N};K(\mathcal{N}\setminus\omega;t)}(t)}\end{aligned} \tag{S77}$$

Eq. (S77) explicitly provides the minimum additional EP rate that must be paid due to the interactions $\phi$ has within a larger dependency structure. It is a lower bound on the minimum difference in the EP rate for the entire system and the EP rate for a unit $\phi \subset \omega$ in that system using thermodynamic quantities under counterfactual rate matrices. This can also be interpreted as an upper bound on the thermodynamically allowable instantaneous (inverse activity-weighted) changes in the distributions of unit $\omega$ and the entire system $\mathcal{N}$ under counterfactual rate matrices.

These results relate *actual* EP rates and learning rates to entirely *counterfactual* thermodynamic quantities, which implies that in multipartite systems, what could be the case *but is not actually happening* has an effect on what *is actually happening* in the system. We note that, while the LHS of Eqs. (S76) and (S77) can be integrated over time, the RHS cannot, due to the reasoning discussed in Fig. S3.

Finally, we note that because the decomposition considered here is iterative, many valid equations such as Eq. (S65) exist in an MPP [12]. Therefore, in general, for any given MPP, there exist very many results analogous to those shown in Eqs. (S75), (S76), and (S77). As one example, the analogous result to Eq. (S75) as applied to the decomposition in Eq. (15) from [12] is

$$\begin{aligned}\langle\dot{\sigma}^{\omega}(t)\rangle - \frac{d^{\phi}}{dt}S^{X_\omega|X_\phi}(t) \geq \\ + \frac{\left(\dot{\mathcal{L}}(p_{x_\phi}(t))\right)^2}{2\mathcal{A}^{\phi}(t)} + \frac{\left(\dot{\mathcal{L}}^{K(\omega\setminus\phi;t)}(p_{x_\omega}(t))\right)^2}{2\mathcal{A}^{\omega;K(\omega\setminus\phi;t)}(t)}\end{aligned} \tag{S78}$$

which is a lower bound on how much greater the local EP rate of $\omega$ must be than the rate at which the subsystems in $\phi$ learn about the subsystems in $\omega\setminus\phi$ (the $\phi-\omega$ learning rate) based on counterfactual instantaneous thermodynamic quantities.

A wealth of other lower bounds can also be derived. As a final example, instead of replacing the $\phi$-local EP rate with its lower bound, we can move it to the LHS to obtain a lower bound on how much greater the *difference* between the $\omega$-local and $\phi$-local EP rates must be than the $\phi-\omega$ learning rate:

$$\Big(\langle\dot\sigma^{\omega}(t)\rangle-\langle\dot\sigma^{\phi}(t)\rangle\Big)-\frac{d^{\phi}}{dt}S^{X_\omega|X_\phi}(t)\geq\frac{\left(\dot{\mathcal{L}}^{K(\omega\setminus\phi;t)}(p_{x_\omega}(t))\right)^2}{2\mathcal{A}^{\omega;K(\omega\setminus\phi;t)}(t)}\tag{S79}$$

# S11 Table of Notation

In Table 1, we collect all the notation used in the main text and explain their meaning in words.

# References


[1] Rory A Brittain, Nick S Jones, and Thomas E Ouldridge. What we learn from the learning rate. *Journal of Statistical Mechanics: Theory and Experiment*, 2017(6):063502, 2017.

[2] David Hartich, Andre C. Barato, and Udo Seifert. Sensory capacity: An information theoretical measure of the performance of a sensor. *Physical Review E*, 93(2), Feb 2016.

[3] Jordan M Horowitz. Multipartite information flow for multiple maxwell demons. *Journal of Statistical Mechanics: Theory and Experiment*, 2015(3):P03006, 2015.

[4] Jordan M Horowitz and Massimiliano Esposito. Thermodynamics with continuous information flow. *Physical Review X*, 4(3):031015, 2014.

[5] Sosuke Ito and Takahiro Sagawa. Information thermodynamics on causal networks. *Physical Review Letters*, 111(18):180603, 2013.

[6] Kangqiao Liu, Zongping Gong, and Masahito Ueda. Thermodynamic uncertainty relation for arbitrary initial states. *Physical Review Letters*, 125(14), Sep 2020.

[7] Sarah AM Loos and Sabine HL Klapp. Irreversibility, heat and information flows induced by non-reciprocal interactions. *New Journal of Physics*, 22(12):123051, 2020.

[8] Takahiro Sagawa and Masahito Ueda. Minimal energy cost for thermodynamic information processing: measurement and information erasure. *Physical review letters*, 102(25):250602, 2009.

[9] Naoto Shiraishi, Ken Funo, and Keiji Saito. Speed limit for classical stochastic processes. *Physical Review Letters*, 121(7), 8 2018.

[10] Naoto Shiraishi and Takahiro Sagawa. Fluctuation theorem for partially masked nonequilibrium dynamics. *Phys. Rev. E*, 91:012130, Jan 2015.

[11] Van Tuan Vo, Tan Van Vu, and Yoshihiko Hasegawa. Unified approach to classical speed limit and thermodynamic uncertainty relation. *Physical Review E*, 102(6), 12 2020.

[12] David H Wolpert. Minimal entropy production rate of interacting systems. *New Journal of Physics*, 22(11):113013, 11 2020.

[13] David H. Wolpert. Uncertainty relations and fluctuation theorems for bayes nets. *Physical Review Letters*, 125(20), Nov 2020.

[14] David H Wolpert. Fluctuation theorems for multiple systems with interdependent dynamics. *New Journal of Physics*, 2021.

| MPP Notation | Meaning in words |
|---|---|
| $\mathcal{N}$ | The global system, composed of a set of $N$ subsystems. |
| $A$; $-A$; $B\backslash A$ | A set of subsystems $A \subseteq \mathcal{N}$; the set of subsystems in $\mathcal{N}$ but not in $A$; the set of subsystems in $B$ but not in $A$. |
| $X$; $x$; $p_x$ | The joint state space of the global system; a particular global state vector; the distribution over the global state space. |
| $X_A$; $x_A$; $p_{x_A}$ | The joint state space of a set $A \subseteq \mathcal{N}$ of subsystems; a particular marginal state vector; the distribution over this state space. |
| $x_{A,-A}$ | Another way to denote $x_{\mathcal{N}}$, with attention called out to the specific states of $A$ and $-A$. |
| $K_x^{x'}(t)$ | The global system's time-$t$ rate of transition from state $x'$ to state $x$. |
| $K_{x_\omega}^{x'_\omega}(t)$ | The unit $\omega$'s time-$t$ rate of transition from state $x'_\omega$ to state $x_\omega$. |
| $\mathcal{N}^*$ | A set of units that covers $\mathcal{N}$ and is closed under intersections, or a unit structure. A single MPP can have more than one valid unit structure. |
| $\mathcal{N}^{**}$ | The collection of all units in $\mathcal{N}$, *other than* the entire system itself. |
| $\mathcal{N}^\dagger$ | $\mathcal{N}^{**} \cup \mathcal{N}$. The collection of all units in $\mathcal{N}$, *including* than the entire system itself. |
| $\tau$ | The given "final" time of system evolution; it can be chosen to be any positive real number. |
| $\mathcal{L}(p_x(0), p_x(\tau))$ | The total variation distance, or L-1 norm, between the initial (time-0) and final (time-$\tau$) global distributions. |
| $\mathcal{L}(p_{x_\omega}(0), p_{x_\omega}(\tau))$ | The total variation distance, or L-1 norm, between the initial (time-0) and final (time-$\tau$) local marginal distributions for unit $\omega$. |
| $\mathcal{L}(p_{x_i}(0), p_{x_i}(\tau))$ | The total variation distance, or L-1 norm, between the initial (time-0) and final (time-$\tau$) local marginal distributions for subsystem $i$. |
| $\langle \sigma^{\mathcal{N}}(\tau) \rangle$ | The total global EP accumulated during the time interval $[0, \tau]$. |
| $\langle \dot{\sigma}^{\mathcal{N}}(t) \rangle$ | The (global) EP rate of the entire system at time $t$. |
| $\langle \mathcal{A}^{\mathcal{N}} \rangle_\tau$ | The time-averaged global dynamical activity (often interpreted as the frequency of state transitions) during the time interval $[0, \tau]$. |
| $\langle \sigma^{\omega}(\tau) \rangle$ | The total local EP accumulated by unit $\omega$ during the time interval $[0, \tau]$. |
| $\langle \dot{\sigma}^{\omega}(t) \rangle$ | The local EP rate of the unit $\omega$ at time $t$. |
| $\langle \mathcal{A}^{\omega} \rangle_\tau$ | The time-averaged local dynamical activity (often interpreted as the frequency of state transitions) for unit $\omega$ during the time interval $[0, \tau]$. |
| $\langle \zeta^i_{\mathcal{N}}(\tau) \rangle$ | The contribution to the total global EP during the time interval $[0, \tau]$ due to (the state transitions in) subsystem $i$. |
| $\langle \dot{\zeta}^i_{\mathcal{N}}(t) \rangle$ | The contribution to the global EP rate at time $t$ due to (the state transitions in) subsystem $i$. |
| $\langle \mathcal{A}^i \rangle_\tau$ | The contribution to the time-averaged dynamical activity (of any unit $\omega \in \mathcal{N}^\dagger$) during the time interval $[0, \tau]$ due to (the state transitions in) subsystem $i$. |
| $\langle \zeta^i_{\omega}(\tau) \rangle$ | The contribution to the total $\omega$-local EP during the time interval $[0, \tau]$ due to (the state transitions in) subsystem $i$. |
| $\langle \dot{\zeta}^i_{\omega}(t) \rangle$ | The contribution to the $\omega$-local EP rate at time $t$ due to (the state transitions in) subsystem $i$. |
| $\langle \vec{\zeta}_{\mathcal{N}}(t) \rangle$ | The vector whose components are $\langle \zeta^i_{\mathcal{N}}(t) \rangle$ for each $i \in \mathcal{N}$. |
| $\langle \vec{\zeta}_{\omega}(t) \rangle$ | The vector whose components are $\langle \zeta^i_{\omega}(t) \rangle$ for each $i \in \omega$. |
| $\langle \vec{\mathcal{A}}_{\mathcal{N}} \rangle_t$ | The vector whose components are $\langle \mathcal{A}^i \rangle_t$ for each $i \in \mathcal{N}$. |
| $\langle \vec{\mathcal{A}}_{\omega} \rangle_t$ | The vector whose components are $\langle \mathcal{A}^i \rangle_t$ for each $i \in \omega$. |

Table 1: Table of Notational Meanings for MPPs
